# Supplementary material for: Choosing The Best Interpolation Data in Images with Noise
Source: arXiv:2011.02363 source file (2020-11-04)
Supplement: Supplementary file 1 [file appendix03.tex]

\section{Draft}
\subsection{Draft}

First, we consider the following homogeneous problem : \\

\begin{problem} Find $w$ in $H^1_0(B(x_0,\varepsilon))$ such that
	\begin{equation}
		\left\{\begin{array}{rl}
			w - \delta t \Delta w = 0, & \text{in}\ B(x_0,\varepsilon), \\
			w = 0, & \text{on}\ \partial B(x_0,\varepsilon).
		\end{array}\right .
	\end{equation}
\end{problem}

We have, \\

\begin{proposition}
    We set for $x$ in $\overline{B(x_0,\varepsilon)}$, $x\neq x_0$,
	
	\[ w(x) := \frac{1}{2\pi}K_0\Big(\frac{|x_0-x|}{\sqrt{\delta t}}\Big) - \frac{1}{2\pi}\frac{K_0\big(\frac{\varepsilon}{\sqrt{\delta t}}\big)}{I_0\big(\frac{\varepsilon}{\sqrt{\delta t}}\big)} I_0\Big(\frac{|x_0-x|}{\sqrt{\delta t}}\Big). \]
	
	The $w$ is a solution of Problem x.
\end{proposition}
\begin{proof}
    \textbullet ~ In polar coordinates : 
    
    \begin{equation}
		\left\{\begin{array}{rl}
			w(r, \theta) - \delta t \big(\partial_{rr}w(r, \theta) + \frac{1}{r}\partial_r w(r, \theta) + \frac{1}{r^2}\partial_{\theta\theta} w(r, \theta) \big) = 0, & \text{for}\ (r, \theta)\in ]0,\varepsilon[\times [0,2\pi[, \\
			w(r, \theta) = 0, & \text{for}\ (r, \theta)\in \{\varepsilon\}\times [0,2\pi[
		\end{array}\right .
	\end{equation}
	
	\textbullet ~ Separation of variables : We suppose that $w = R(r)\Theta(\theta)$. Thus, for $(r, \theta)\in ]0,\varepsilon[\times [0,2\pi[$, we have,
	
	\[ w(r, \theta) - \delta t \big(\partial_{rr}w(r, \theta) + \frac{1}{r}\partial_r w(r, \theta) + \frac{1}{r^2}\partial_{\theta\theta} w(r, \theta) \big) = 0 \]
	
	\[ R(r)\Theta(\theta) - \delta t R''(r)\Theta(\theta) - \frac{\delta t}{r}R'(r)\Theta(\theta) - \frac{\delta t}{r^2} R(r)\Theta''(\theta) = 0 \]
	
	\[ r^2 - r^2\delta t \frac{R''(r)}{R(r)} - r \delta t \frac{R'(r)}{R(r)} = \delta t \frac{\Theta''(\theta)}{\Theta(\theta)} = \lambda \]
	
	\[ \left\{\begin{array}{l}
		r^2 R''(r) + r R'(r) - \frac{1}{\delta t}(r^2 - \lambda) R(r) = 0, \\
		\Theta''(\theta) - \frac{\lambda}{\delta t} \Theta(\theta) = 0.
	\end{array}\right . \]
	
	\textbullet ~ Solve $\Theta''(\theta) - \frac{\lambda}{\delta t} \Theta(\theta) = 0$. EDO ordre 2 à coeff constants. We set $\Delta := \frac{4 \lambda}{\delta t}$.
	
	\hspace{1cm} -- ~ If $\Delta = 0$ (i.e. $\lambda = 0$) :
	
	\[ \Theta(\theta) = (A\theta + B),\ \text{for}\ (A,B)\in\R^2. \]
	
	However, in polar coordinates, we want $\Theta$ to be $2\pi$-periodic. In this case, it is possible if and only if $A=0$. Then the solution is 
	
	\[ \Theta(\theta) = B,\ \text{for}\ B\in\R. \]
	
	\hspace{1cm} -- ~ If $\Delta > 0$ (i.e. $\lambda > 0$) :
	
	\[ \Theta(\theta) = Ae^{\sqrt{\frac{\lambda}{\delta t}}\theta} + Be^{-\sqrt{\frac{\lambda}{\delta t}} \theta},\ \text{for}\ (A,B)\in\R^2. \]
	
	Again, in polar coordinates, we want $\Theta$ to be $2\pi$-periodic, which is not the case for $\lambda > 0$. Thus, this case is impossible.
	
	\hspace{1cm} -- ~ If $\Delta < 0$ (i.e. $\lambda < 0$), we set $\nu^2 := (i\sqrt{\frac{|\lambda|}{\delta t}})^2$. Then,
	
	\[ \Theta(\theta) = A\cos\Big(\sqrt{\frac{|\lambda|}{\delta t}}\theta\Big) + B\sin\Big(\sqrt{\frac{|\lambda|}{\delta t}}\theta\Big),\ \text{for}\ (A,B)\in\R^2.\]
	
	\textbullet ~ Solve $r^2 R''(r) + r R'(r) - \frac{1}{\delta t}(r^2 - \lambda) R(r) = 0$. We set $x := \frac{r}{\sqrt{\delta t}}$ and $y(x) := R(\sqrt{\delta t} x)$. The equation become $x^2 y''(x) + x y'(x) - (x^2 - \frac{\lambda}{\delta t}) y(x) = 0$. This equation is known as the modified Bessel's equation.
	
	%\hspace{1cm} -- ~ If $\lambda = 0$ : Solve $x y''(x) + y'(x) - xy(x) = 0$ which can be rewritten $\big(x y'(x)\big)' = xy(x)$.
	
	\hspace{1cm} -- ~ If $\lambda \leq 0$ : Solve $x^2 y''(x) + x y'(x) - (x^2 + \frac{|\lambda|}{\delta t}) y(x) = 0$. Setting $\nu := \sqrt{\frac{|\lambda|}{\delta t}}$, the equation became $x^2 y''(x) + x y'(x) - (x^2 + \nu^2) y(x) = 0$. Using the Frobenius' method, one can show that
	
	\[ y(x) = AI_\nu(x) + BK_\nu(x),\ \text{for}\ (A,B)\in\R^2, \]
	
	where $I_\nu$ is a modified Bessel function of the first kind and $K_\nu$ is a modified Bessel function of the second kind. Therefore,  
	\[ R(r) = AI_\nu\Big(\frac{r}{\sqrt{\delta t}}\Big) + BK_\nu\Big(\frac{r}{\sqrt{\delta t}}\Big),\ \text{for}\ (A,B)\in\R^2. \]
	
	To sum up, we have for $\lambda \leq 0$,
	
	\[ w(r,\theta) = \Big(C\cos(\nu\theta) + D\sin(\nu\theta)\Big)\Big(AI_\nu\big(\frac{r}{\sqrt{\delta t}}\big) + BK_\nu\big(\frac{r}{\sqrt{\delta t}}\big)\Big),\ \text{for}\ (A,B,C,D)\in\R^4, \]
	
	where $\nu := \sqrt{\frac{|\lambda|}{\delta t}}$.
	
	\textbullet ~ Determining $\lambda$ : The boundary condition gives us, for all $\theta$ in $[0,2\pi[$,
	
	\[ w(\varepsilon,\theta) = \Big(C\cos(\nu\theta) + D\sin(\nu\theta)\Big)\Big(AI_\nu\big(\frac{\varepsilon}{\sqrt{\delta t}}\big) + BK_\nu\big(\frac{\varepsilon}{\sqrt{\delta t}}\big)\Big) = 0. \]

    $AI_\nu\big(\frac{\varepsilon}{\sqrt{\delta t}}\big) + BK_\nu\big(\frac{\varepsilon}{\sqrt{\delta t}}\big) = 0$ $\Leftrightarrow$ $AI_\nu\big(\frac{\varepsilon}{\sqrt{\delta t}}\big) = - BK_\nu\big(\frac{\varepsilon}{\sqrt{\delta t}}\big)$ $\Leftrightarrow$ $A = - B \frac{K_\nu\big(\frac{\varepsilon}{\sqrt{\delta t}}\big)}{I_\nu\big(\frac{\varepsilon}{\sqrt{\delta t}}\big)}$.
	
	\[ w(r,\theta) = \Big(C\cos(\nu\theta) + D\sin(\nu\theta)\Big)B\Big(K_\nu\big(\frac{r}{\sqrt{\delta t}}\big) - \frac{K_\nu\big(\frac{\varepsilon}{\sqrt{\delta t}}\big)}{I_\nu\big(\frac{\varepsilon}{\sqrt{\delta t}}\big)} I_\nu\big(\frac{r}{\sqrt{\delta t}}\big) \Big),\ \text{for}\ D\in\R. \]
	
	In particular, if we take $\lambda = 0$, $B=\frac{1}{2\pi}$, we get
	
	\[ w(r,\theta) = \frac{1}{2\pi}K_0\big(\frac{r}{\sqrt{\delta t}}\big) - \frac{1}{2\pi}\frac{K_0\big(\frac{\varepsilon}{\sqrt{\delta t}}\big)}{I_0\big(\frac{\varepsilon}{\sqrt{\delta t}}\big)} I_0\big(\frac{r}{\sqrt{\delta t}}\big). \]
	
\end{proof}

\begin{proposition}
    \[ w(x) = \frac{1}{2\pi} \ln\Bigg(\frac{\varepsilon}{|x-x_0|}\Bigg) + O\Big(|x-x_0|^2\ln(|x-x_0|)\Big) + O(\varepsilon^2) \]
\end{proposition}
\begin{proof}

    %\[ I_0(z) = \frac{e^z}{\sqrt{2\pi z}} + \frac{e^z}{\sqrt{2\pi z}}\sum_1^\infty \frac{((2j)!)^2}{(j!)^3}\Big(\frac{1}{32 z}\Big)^j \]
    
    \[ I_n(z) = \Big(\frac{x}{2}\Big)^n + \Big(\frac{x}{2}\Big)^n \sum_{j=1}^\infty \frac{\big(\frac{x^2}{4}\big)^j}{j!(j+n)!} = \Big(\frac{x}{2}\Big)^n + O(x^{n+2}). \]

    \[ K_0(z) = -\Big(\gamma + \ln\big(\frac{z}{2}\big)\Big)I_0(z) + 2\sum_1^\infty \frac{I_{2j}(z)}{j} \]
    
    %\[ (pas beau = -\Big(\gamma + \ln\big(\frac{z}{2}\big)\Big) + O(x^2\ln(z)) + 2\sum_1^\infty \Big(\frac{x}{2}\Big)^{2j} + O(x^{2j+2}) ) \]
    
    \[ = -\ln(z) + \ln(2) - \gamma + O(x^2\ln(z)). \]
    
    and 
    
    \[ I_0(z) = 1 + O(x^{2}) \]
    
    Thus 
    
    \[ w(r,\theta) = \frac{1}{2\pi}K_0\big(\frac{r}{\sqrt{\delta t}}\big) - \frac{1}{2\pi}\frac{K_0\big(\frac{\varepsilon}{\sqrt{\delta t}}\big)}{I_0\big(\frac{\varepsilon}{\sqrt{\delta t}}\big)} I_0\big(\frac{r}{\sqrt{\delta t}}\big) \]
    
    \[ = \frac{1}{2\pi}\Bigg(-\ln(r) + \frac{1}{2}\ln(\delta t) + \ln(2) - \gamma - \frac{K_0\big(\frac{\varepsilon}{\sqrt{\delta t}}\big)}{I_0\big(\frac{\varepsilon}{\sqrt{\delta t}}\big)}\Bigg) + O(r^2\ln(r)) \]
    
    \[ = \frac{1}{2\pi} \ln\Big(\frac{\varepsilon}{r}\Big) + O\big(r^2\ln(r)\big) + O(\varepsilon^2) \]
    
\end{proof}

Then, we consider the non-homogeneous problem : \\

\begin{problem} Find $w$ in $H^1_0(B_\varepsilon)$ such that
	\begin{equation}
		\left\{\begin{array}{rl}
			w - \delta t \Delta w = g, & \text{in}\ B_\varepsilon, \\
			w = 0, & \text{on}\ \partial B_\varepsilon.
		\end{array}\right .
	\end{equation}
\end{problem}

We have, \\

\begin{proposition}
    \[ \int_{B_\varepsilon} f-u_\varepsilon\ dx = C \big(f(x_0) - \alpha\Delta f(x_0)\big)\varepsilon^2\ln\varepsilon + O(\varepsilon^2\ln\varepsilon). \]
\end{proposition}
\begin{proof}
    We use the Green function corresponding to Problem 6.4, that is
    
    \begin{problem} Find $N(\cdot,y)$ in $H^1_0(B_\varepsilon)$ such that
    	\begin{equation}
    		\left\{\begin{array}{rl}
    			N(x,y) - \delta t \Delta_x N(x,y) = \delta_y(x), & x\in B_\varepsilon, \\
    			N(x,y) = 0, & x\in\partial B_\varepsilon,
    		\end{array}\right .
    	\end{equation}
    	for $y$ in $B_\varepsilon$.
    \end{problem}
    
    Using Proposition 6.2, we have for $y\in B_\varepsilon$ and $x\in B_\varepsilon$ such that $x\neq y$,
    
    \[ N(x,y) = \begin{cases}
        \frac{1}{2\pi}K_0\Big(\frac{|y-x|}{\sqrt{\delta t}}\Big) - \frac{1}{2\pi}\frac{K_0\big(\frac{\varepsilon-|y-x_0|}{\sqrt{\delta t}}\big)}{I_0\big(\frac{\varepsilon-|y-x_0|}{\sqrt{\delta t}}\big)} I_0\Big(\frac{|y-x|}{\sqrt{\delta t}}\Big)  &,\ \text{if}\ |x-y| \leq \varepsilon-|y-x_0|, \\
        
        0 &,\ \text{if}\ |x-y| > \varepsilon-|y-x_0|.
    \end{cases} \]
    
    and using Proposition 6.3,
    
    \[ N(x,y) = \begin{cases}
        \frac{1}{2\pi} \ln\Big(\frac{\varepsilon-|y-x_0|}{|x-y|}\Big) + O\Big(|x-y|^2\ln(|x-y|)\Big) + O\Big((\varepsilon-|y-x_0|)^2\Big) &,\ \text{if}\ |x-y| \leq \varepsilon-|y-x_0|, \\
        
        0 &,\ \text{if}\ |x-y| > \varepsilon-|y-x_0|.
    \end{cases} \]
    
    \[ w(x) = \int_{B_\varepsilon} N(x,y)g(y)\ dy \]
    
    \[ = \int_{B_\varepsilon} \mathbf{1}_{\big\{ y\in B_\varepsilon\ \big|\ |x-y| \leq \varepsilon-|y-x_0| \big\}}(y) \Bigg(\frac{1}{2\pi} \ln\Big(\frac{\varepsilon-|y-x_0|}{|x-y|}\Big) + O\Big(|x-y|^2\ln(|x-y|)\Big) + O\Big((\varepsilon-|y-x_0|)^2\Big)\Bigg)g(y)\ dy \]
    
    \[ \int_{B_\varepsilon} w(x)\ dx = \int_{B_\varepsilon} \int_{B_\varepsilon} \mathbf{1}_{\big\{ y\in B_\varepsilon\ \big|\ |x-y| \leq \varepsilon-|y-x_0| \big\}}(y) \Bigg(\frac{1}{2\pi} \ln\Big(\frac{\varepsilon-|y-x_0|}{|x-y|}\Big) + O\Big(|x-y|^2\ln(|x-y|)\Big) + O\Big((\varepsilon-|y-x_0|)^2\Big)\Bigg)g(y)\ dy\ dx \]
    
    \[ \leq \frac{1}{2\pi} \int_{B_\varepsilon} \int_{B_\varepsilon}  \ln\Big(\frac{\varepsilon-|y-x_0|}{|x-y|}\Big) g(y)\ dy\ dx + \int_{B_\varepsilon} \int_{B_\varepsilon} O\Big((\varepsilon-|y-x_0|)^2\ln(|\varepsilon-|y-x_0|)\Big) g(y)\ dy\ dx\]
    
    Fubini
    
    \[ \leq \frac{\varepsilon^2}{2} \int_{B_\varepsilon} g(y) \ln\Big(\varepsilon-|y-x_0|\Big)\ dy - \frac{1}{2\pi} \int_{B_\varepsilon} g(y) \int_{B_\varepsilon}  \ln\Big(|x-y|\Big) \ dx\ dy + \pi\varepsilon^2 \int_{B_\varepsilon} O\Big((\varepsilon-|y-x_0|)^2\ln(|\varepsilon-|y-x_0|)\Big) g(y) \ dy\]
    
    Taylor : $g(y) = g(x_0) + |y-x_0|O(1)$
    
    \[ \leq \underbrace{\frac{\varepsilon^2}{2} \int_{B_\varepsilon} g(y) \ln\Big(\varepsilon-|y-x_0|\Big)\ dy}_{=: I_1} - \underbrace{\frac{1}{2\pi} \int_{B_\varepsilon} g(y) \int_{B_\varepsilon}  \ln\Big(|x-y|\Big) \ dx\ dy}_{=: I_2} + \underbrace{\pi\varepsilon^2 \int_{B_\varepsilon} g(y) O\Big((\varepsilon-|y-x_0|)^2\ln(|\varepsilon-|y-x_0|)\Big)\ dy}_{=: I_3} \]
    
    \textbullet ~ $I_1$ : \[ I_1 = \frac{\varepsilon^2}{2} g(x_0) \int_{B_\varepsilon}  \ln\Big(\varepsilon-|y-x_0|\Big)\ dy + \frac{\varepsilon^2}{2} \int_{B_\varepsilon} \ln\Big(\varepsilon-|y-x_0|\Big)O(|y-x_0|)\ dy \]
    
    \[ = \frac{g(x_0)}{2} \varepsilon^3(\ln \varepsilon - 1) + \frac{\varepsilon^2}{2} \int_{B_\varepsilon} \ln\Big(\varepsilon-|y-x_0|\Big)O(|y-x_0|)\ dy \]
    
    \[ = \frac{g(x_0)}{2} \varepsilon^3(\ln \varepsilon - 1) + O(\varepsilon^3 \ln\varepsilon) \]
    
    \[ = \frac{g(x_0)}{2} \varepsilon^3\ln\varepsilon + O(\varepsilon^3 \ln\varepsilon) \]
    
    \textbullet ~ $I_2$ : \[ I_2 = \frac{1}{2\pi} g(x_0) \int_{B_\varepsilon} \int_{B_\varepsilon} \ln\Big(|x-y|\Big) \ dx\ dy + \frac{1}{2\pi} \int_{B_\varepsilon} O(|y-x_0|) \int_{B_\varepsilon} \ln\Big(|x-y|\Big) \ dx\ dy \]
    
    \[ = C g(x_0)\varepsilon^2\ln\varepsilon + O(\varepsilon^2\ln\varepsilon) \]
    
    \textbullet ~ $I_3$ : \[ I_3 = \pi\varepsilon^2 g(x_0) \int_{B_\varepsilon} O\Big((\varepsilon-|y-x_0|)^2\ln(|\varepsilon-|y-x_0|)\Big) \ dy + \pi\varepsilon^2 \int_{B_\varepsilon} O\Big(|y-x_0|(\varepsilon-|y-x_0|)^2\ln(|\varepsilon-|y-x_0|)\Big) \ dy \]
    
    \[ = \pi g(x_0) O(\varepsilon^5\ln\varepsilon) + \pi O(\varepsilon^6\ln\varepsilon) \]
    
    \[ = O(\varepsilon^5\ln\varepsilon) \]
    
\end{proof}

\begin{proposition}
    
\end{proposition}
\begin{proof}
    \[ G(r_x, \theta_x, r_y, \theta_y) - \alpha\partial_{r_xr_x}G(r_x, \theta_x, r_y, \theta_y) - \alpha\frac{1}{r_x}\partial_{r_x} G(r_x, \theta_x, r_y, \theta_y) - \alpha\frac{1}{r_x^2}\partial_{\theta_x\theta_x} G(r_x, \theta_x, r_y, \theta_y) = \delta_0(r_y - r_x)\delta_0(\theta_y-\theta_x). \]
    
    Like in [Green’s Functions with Applications, Second Edition p.450], we proceed by separation of variable, i.e. we assume 
    
    \[ G(r_x, \theta_x, r_y, \theta_y) = \sum_{n=-\infty}^{+\infty} G_n(r_x,r_y) \cos\big(n(\theta_y-\theta_x)\big). \]
    
    Moreover, since $\delta_0(\theta_y-\theta_x)$ is $2\pi$-periodic, Fourier expansion gives us
    
    \[ \delta_0(\theta_y-\theta_x) = \frac{1}{2\pi} + \frac{1}{\pi}\sum_{k=1}^{+\infty}\cos\big(n(\theta_y-\theta_x)\big) = \frac{1}{2\pi}\sum_{k=-\infty}^{+\infty}\cos\big(n(\theta_y-\theta_x)\big). \]
    
    Thus, we have, by setting for simplicity $G_n(\cdot) := G_n(\cdot,r_y)$,
    
    \[ \sum_{n=-\infty}^{+\infty} \big( \alpha G_n''(r_x) + \alpha\frac{1}{r_x}G_n'(r_x) - (1 + \alpha\frac{n^2}{r_x^2})G_n(r_x) \big) \cos\big(n(\theta_y-\theta_x)\big) = \sum_{k=-\infty}^{+\infty}\frac{-\delta_0(r_y - r_x)}{2\pi}\cos\big(n(\theta_y-\theta_x)\big). \]
    
    Using the uniqueness of Fourier expansion, it comes
    
    \[ r_x^2 G_n''(r_x) + r_x G_n'(r_x) - \frac{1}{\alpha}\Big(r_x^2 + \alpha n^2 \Big)G_n(r_x) = \frac{-\delta_0(r_y - r_x)}{2\pi\alpha}. \]
    
    The solution of the homogeneous equation $G_n^0$ is given by proposition x, i.e. (n/sqrt alpha ?)
    
    \[ G_n^0(r_x) = AI_n \Big(\frac{r_x}{\sqrt{\alpha}}\Big) + BK_n \Big(\frac{r_x}{\sqrt{\alpha}}\Big),\ \text{for}\ (A,B)\in\R^2. \]
    
    For $r_y\neq r_x$, a solution $G_n^\text{p}$ is given by
    
    \[ G_n^\text{p}(r_x) = -\frac{1}{2\pi}K_0(\alpha|r_x-r_y|). \]
    
    Indeed, $G_n^\text{p}$ satisfies the homogeneous equation for $r_x\neq r_y$ and we have also
    
    \[ \lim_{\delta\to 0} \Delta G_n^\text{p}(r+\delta) + \alpha G_n^\text{p}(r+\delta) = \delta_0(r). \]
    
    Then the Green function for x is given by
    
    \[ G(r_x,r_y) = -\frac{1}{2\pi}K_0(\alpha|r_x-r_y|) + G_n^0(r_x,r_y), \]
    
    with $G_n^0(\varepsilon,r_y) = \frac{1}{2\pi}K_0(\alpha|\varepsilon-r_y|)$
    
\end{proof}

\section{Draft 2}

In this section, we aim to find an analytic solution of the problem below : \\

\begin{problem} Find $w$ in $H^1_0(B_\varepsilon)$ such that
	\begin{equation}
		\left\{\begin{array}{rl}
			w - \alpha \Delta w = g, & \text{in}\ B_\varepsilon, \\
			w = 0, & \text{on}\ \partial B_\varepsilon.
		\end{array}\right .
	\end{equation}
\end{problem}

To solve Problem 7.1, we use Green functions $G:B_\varepsilon\times B_\varepsilon$, corresponding to Problem 7.1 which are solution to \\

\begin{problem} Find $G(\cdot,y)$ in $H^1_0(B_\varepsilon)$ such that
    \begin{equation}
    	\left\{\begin{array}{rl}
    		G(x,y) - \alpha \Delta_x G(x,y) = \delta_y(x), & x\in B_\varepsilon, \\
    		G(x,y) = 0, & x\in\partial B_\varepsilon,
    	\end{array}\right .
    \end{equation}
    for $y$ in $B_\varepsilon$.
\end{problem}

We have, \\

\begin{proposition}
    Let $G$ be Green functions corresponding to Problem 7.1. Then, for $x$ in  $\bar{B_\varepsilon}$,
    
    \[ w(x) := \int_{B_\varepsilon} g(y)G(x,y)\ dy, \]
    
    is the solution of Problem 7.1.
\end{proposition}
\begin{proof}
    Let $x$ be in $B_\varepsilon$.
    
    \begin{align*}
        w(x) - \alpha \Delta w(x) &= \int_{B_\varepsilon} g(y)G(x,y)\ dy - \alpha \int_{B_\varepsilon} g(y)\Delta_x G(x,y)\ dy \\
            &= \int_{B_\varepsilon} g(y)\big(G(x,y) - \alpha\Delta_x G(x,y)\big)\ dy \\
            &= \int_{B_\varepsilon} g(y)\delta_y(x)\ dy \\
            &= g(x).
    \end{align*}
    
    Moreover, we have,  $w(x)=0$, for $x$ on $\partial D_\varepsilon$.
\end{proof}

From now, our goal is to find Green functions $G$. To do so, we write $G$ as the sum of a particular solution $G_\text{p}$ of Problem 7.2 without the boundary condition, and the general solution $G_0$ of the homogeneous version of Problem 7.2 such that $G_0 = -G_\text{p}$ on $\partial B_\varepsilon$. \\

\begin{proposition} For $x$ and $y$ in $B_\varepsilon$ such that $x\neq y$, we have
    \[ G_\text{p}(x,y) = \frac{1}{2\pi}K_0\Big(\frac{1}{\sqrt{\alpha}}|x-y|\Big), \]
    
    where $K_0$ is the modified Bessel function of the second kind, see [An Atlas of Functions].
\end{proposition}
\begin{proof}
    TODO
\end{proof}

\begin{proposition} For $x$ in $B_\varepsilon$, we have
    \[ G_0(r_x,\theta_x,r_y,\theta_y) = -\frac{1}{2\pi}\sum_{n=-\infty}^{+\infty} \frac{I_n(\frac{r_y}{\sqrt{\alpha}}) K_n(\frac{\varepsilon}{\sqrt{\alpha}})}{I_n \Big(\frac{\varepsilon}{\sqrt{\alpha}}\Big)} I_n \Big(\frac{r_x}{\sqrt{\alpha}}\Big)\cos(n(\theta_y-\theta_x)), \]
    
    where $I_0$ is a modified Bessel function of the first kind and $K_0$ is a modified Bessel function of the second kind, see [An Atlas of Functions].
\end{proposition}
\begin{proof}
    \textbullet ~ First, we write our homogeneous problem in polar coordinates. For $(r, \theta)$ in $]0,\varepsilon[\times [0,2\pi[$, we want to solve
    
    \[ G_0(r, \theta) - \alpha \big(\partial_{rr}G_0(r, \theta) + \frac{1}{r}\partial_r G_0(r, \theta) + \frac{1}{r^2}\partial_{\theta\theta} G_0(r, \theta) \big) = 0. \]
    
    \textbullet ~ Then, we proceed by separation of variables i.e. we suppose that $G_0 = R(r)\Theta(\theta)$. Thus, for $(r, \theta)\in ]0,\varepsilon[\times [0,2\pi[$, we have,
	
	\[ G_0(r, \theta) - \alpha \big(\partial_{rr}G_0(r, \theta) + \frac{1}{r}\partial_r G_0(r, \theta) + \frac{1}{r^2}\partial_{\theta\theta} G_0(r, \theta) \big) = 0 \]
	
	\[ R(r)\Theta(\theta) - \alpha R''(r)\Theta(\theta) - \frac{\alpha}{r}R'(r)\Theta(\theta) - \frac{\alpha}{r^2} R(r)\Theta''(\theta) = 0 \]
	
	\[ r^2 - r^2\alpha\frac{R''(r)}{R(r)} - r \alpha \frac{R'(r)}{R(r)} = \alpha \frac{\Theta''(\theta)}{\Theta(\theta)} = -\lambda \]
	
	\[ \left\{\begin{array}{l}
		r^2 R''(r) + r R'(r) - \frac{1}{\alpha}(r^2 + \lambda) R(r) = 0, \\
		\Theta''(\theta) + \frac{\lambda}{\alpha} \Theta(\theta) = 0.
	\end{array}\right . \]
	
	\textbullet ~ Now, we solve $\Theta''(\theta) + \frac{\lambda}{\alpha} \Theta(\theta) = 0$. We set $\Delta := -\frac{4 \lambda}{\alpha}$. Since we want $\Theta$ to be $2\pi$-periodic, we have to impose $\lambda > 0$ and $\Theta(\theta) = A\cos\Big(\sqrt{\frac{\lambda}{\alpha}}\theta\Big) + B\sin\Big(\sqrt{\frac{\lambda}{\alpha}}\theta\Big)$, $(A,B)\in\R^2$ or $\lambda = 0$ and $\Theta$ is constant. Thus we have,
	
	\[ \Theta(\theta) = A\cos\Big(\sqrt{\frac{\lambda}{\alpha}}\theta\Big) + B\sin\Big(\sqrt{\frac{\lambda}{\alpha}}\theta\Big),\ \text{for}\ (A,B)\in\R^2, \]
	
	for $\lambda \geq 0$.
	
	\textbullet ~ After that, we solve $r^2 R''(r) + r R'(r) - \frac{1}{\alpha}(r^2 + \lambda) R(r) = 0$. We set $x := \frac{r}{\sqrt{\alpha}}$ and $y(x) := R(\sqrt{\alpha} x)$. The equation become $x^2 y''(x) + x y'(x) - (x^2 + \frac{\lambda}{\alpha}) y(x) = 0$. This equation is known as the modified Bessel's equation. Using the Frobenius' method, one can show that
	
	\[ y(x) = AI_{\sqrt{\lambda/\alpha}}(x) + BK_{\sqrt{\lambda/\alpha}}(x),\ \text{for}\ (A,B)\in\R^2, \]
	
	where $I_{\sqrt{\lambda/\alpha}}$ is a modified Bessel function of the first kind and $K_{\sqrt{\lambda/\alpha}}$ is a modified Bessel function of the second kind. Therefore,  
	
	\[ R(r) = AI_{\sqrt{\lambda/\alpha}}\Big(\frac{r}{\sqrt{\alpha}}\Big) + BK_{\sqrt{\lambda/\alpha}}\Big(\frac{r}{\sqrt{\alpha}}\Big),\ \text{for}\ (A,B)\in\R^2. \]
	
	\textbullet ~ Finally, we have to determine the constants. The boundary condition gives us 
	
	\[ G_0(\varepsilon,\theta) = -G_p(\varepsilon, \theta) \]
	\[ = - \frac{1}{2\pi}K_0\Big(\frac{\sqrt{r_y^2+\varepsilon^2 - 2r_y \varepsilon\cos(\theta_y - \theta)}}{\sqrt{\alpha}}\Big) \]
	
	The addition theorem for Bessel functions [ref], gives us (?)
	
	\[ G_p(r_x, \theta_y, r_y, \theta_y) = \frac{1}{2\pi}\sum_{n=-\infty}^{+\infty} I_n(\frac{r_y}{\sqrt{\alpha}}) K_n(\frac{r_x}{\sqrt{\alpha}})\cos(n(\theta_y-\theta_x)) \]
	
	Since our problem is linear, we have also for solution
	
	\[ G_0^\infty = \sum_{n=-\infty}^{+\infty}\bigg(A(r_y,\theta_y)\cos\Big(n\theta_x\Big) + B(r_y,\theta_y)\sin\Big(n\theta_x\Big)\bigg)\bigg( C(r_y,\theta_y)I_n \Big(\frac{r_x}{\sqrt{\alpha}}\Big) + D(r_y,\theta_y)K_n \Big(\frac{r_x}{\sqrt{\alpha}}\Big)\bigg) \]
	
	In particular, for 
	\[ A(r_y,\theta_y) = \cos(n\theta_y) \]
	\[ B(r_y,\theta_y) = \sin(n\theta_y) \]
	\[ C(r_y,\theta_y) = -\frac{1}{2\pi}\frac{I_n(\frac{r_y}{\sqrt{\alpha}}) K_n(\frac{\varepsilon}{\sqrt{\alpha}})}{I_n \Big(\frac{\varepsilon}{\sqrt{\alpha}}\Big)} \]
	\[ D(r_y,\theta_y) = 0 \]
	
	we have,
	
	\[ G_0^\infty(\varepsilon, \theta_y, r_y, \theta_y) = -G_p(\varepsilon, \theta_y, r_y, \theta_y) \]
	
	and
	
	\[ G_0^\infty = -\frac{1}{2\pi}\sum_{n=-\infty}^{+\infty} \frac{I_n(\frac{r_y}{\sqrt{\alpha}}) K_n(\frac{\varepsilon}{\sqrt{\alpha}})}{I_n \Big(\frac{\varepsilon}{\sqrt{\alpha}}\Big)} I_n \Big(\frac{r_x}{\sqrt{\alpha}}\Big)\cos(n(\theta_y-\theta_x)) \]
	
	To conclude, $G_0 = G_0^\infty$;
	
\end{proof}

\subsection{strat 1}

\begin{proposition} For $x$ and $y$ in $B_\varepsilon$ such that $|x-y|\to 0$,
    \[ G(x,y) = -\frac{1}{2\pi}\Big(\ln|x-y| + \frac{1}{2}\ln \alpha + \ln 2 - \gamma\Big) + O\Big(|x-y|^2|\ln|x-y||\Big) + O\Big( \frac{\varepsilon^2}{\varepsilon^2 - |x-x_0||y-y_0|}\Big), \]
    
    when $\varepsilon\to 0$, where $\gamma$ denotes the Euler–Mascheroni constant.
\end{proposition}
\begin{proof}
    \textbullet ~ According to [Atlas of function?], we have 
    
    \[ K_0(z) = -\ln z + \ln 2 - \gamma + O(z^2|\ln z|), \]
    
    for $z\to 0$, where $\gamma$ denotes the Euler–Mascheroni constant. Then,
    
    \[ G_\text{p}(x,y) = -\frac{1}{2\pi}\Big(\ln|x-y| + \frac{1}{2}\ln \alpha + \ln 2 - \gamma\Big) + O(|x-y|^2|\ln|x-y||), \]
    
    for $|x-y|\to 0$.
    
    \textbullet ~ 
    
    \[ G_0(r_x,\theta_x,r_y,\theta_y) = -\frac{1}{2\pi}\sum_{n=-\infty}^{+\infty} \frac{I_n(\frac{r_y}{\sqrt{\alpha}}) K_n(\frac{\varepsilon}{\sqrt{\alpha}})}{I_n \Big(\frac{\varepsilon}{\sqrt{\alpha}}\Big)} I_n \Big(\frac{r_x}{\sqrt{\alpha}}\Big)\cos(n(\theta_y-\theta_x)), \]
    
    From [Atlas of functions], we have when $z\to 0$,
    
    \[ K_n(z) = \frac{(n-1)!}{2}\sum_{k=0}^{n-1} \frac{(z/2)^{2k-n}}{(1)_k(1-n)_k} + \frac{1}{n!}(\frac{-z}{2})^n\sum_{j=0}^{+\infty}(\frac{\Psi(j+1)+\Psi(n+j+1)}{2} - \ln(\frac{z}{2}))\frac{(z^2/4)^j}{(1)_j(n+1)_j} = \begin{cases} O(z^{-n}) & \text{if}\ n\geq 0 \\ O(z^n) & \text{if}\ n<0 \end{cases}, \]
    
    and
    
    \[ I_n(z) = \frac{(z/2)^n}{\Gamma(1+n)}\sum_{j=0}^{+\infty} \frac{1}{(1+n)_j (1)_j}(\frac{z^2}{4})^j = O(z^n). \]
    
    Then
    
    \[ G_0(r_x,\theta_x,r_y,\theta_y) = \sum_{n=0}^{+\infty}\Bigg[ O\Bigg(\Big(\frac{1}{r_y r_x}\Big)^n\Bigg) + O\Bigg(\Big(\frac{r_y r_x}{\varepsilon^2}\Big)^n\Bigg) \Bigg] = \sum_{n=0}^{+\infty} O\Bigg(\Big(\frac{r_y r_x}{\varepsilon^2}\Big)^n\Bigg) = \lim_{N\to+\infty} \sum_{n=0}^{N} O\Bigg(\Big(\frac{r_y r_x}{\varepsilon^2}\Big)^n\Bigg) \]
    
    \[ = \lim_{N\to+\infty} O\Bigg(\frac{1-\Big(\frac{r_y r_x}{\varepsilon^2}\Big)^N}{1-\frac{r_y r_x}{\varepsilon^2}}\Bigg) = O\Bigg( \frac{\varepsilon^2}{\varepsilon^2 - r_y r_x}\Bigg). \]
\end{proof}

\begin{proposition}
    Let $G$ be Green functions corresponding to Problem 7.1. Then, for $x$ in  $\bar{B_\varepsilon}$,
    
    \[ w(x) = ?. \]
\end{proposition}
\begin{proof}
    Let $x$ be in $B_\varepsilon$. From Proposition x, we have,
    
    \[ w(x) = \int_{B_\varepsilon} g(y)G(x,y)\ dy. \]
    
    Taylor's formula leads to
    
    \[ w(x) = g(x_0) \int_{B_\varepsilon} G(x,y)\ dy + O(1) \int_{B_\varepsilon} \|y-x_0\|G(x,y)\ dy \]
    
    \[ = g(x_0) \int_0^{2\pi} \int_0^\varepsilon r G(x,(r,\theta))\ dr\ d\theta + O(1) \int_0^{2\pi} \int_0^\varepsilon r^2 G(x,(r,\theta))\ dr\ d\theta \]
    
    \textbullet ~ 1
    \[ O(1) \int_0^{2\pi} \int_0^\varepsilon r \frac{\varepsilon^2}{\varepsilon^2 - |x-x_0|r}\ dr\ d\theta = -\pi\varepsilon|x-x_0|O(1) -\pi\varepsilon^2 \ln(|\frac{|x-x_0|}{\varepsilon} - 1|)O(1) = O\big( \varepsilon^2 \ln|\frac{|x-x_0|}{\varepsilon} - 1| \big) \]
    
    \[ = O\big( \varepsilon^2 \ln\frac{1}{\varepsilon}||x-x_0| - \varepsilon| \big) = O\big( \varepsilon^2 \ln||x-x_0| - \varepsilon| \big) - O\big( \varepsilon^2 \ln\varepsilon \big) = O\big( \varepsilon^2 \ln||x-x_0| - \varepsilon| \big) \]
    
    \textbullet ~ 2 (TODO)
    
    \[ -\frac{1}{2\pi}\int_0^{2\pi} \int_0^\varepsilon r \ln\sqrt{r_x^2+r^2-2r_x r\cos(\theta_x-\theta)}\ dr\ d\theta = -\frac{1}{4\pi}\int_0^{2\pi} \int_0^\varepsilon r \ln(r_x^2+r^2-2r_x r\cos(\theta_x-\theta))\ dr\ d\theta\]
    
    \[ = -\frac{1}{4\pi}\int_0^{2\pi}  [\frac{r^2}{2}\ln(r_x^2+r^2-2r_x r\cos(\theta_x-\theta))]_0^\varepsilon - \int_0^\varepsilon \frac{r^2}{2}\frac{2r-2r_x  r\cos(\theta_x-\theta)}{r_x^2+r^2-2r_x r\cos(\theta_x-\theta)} \ dr\ d\theta\]
    
    \[ = -\frac{\varepsilon^2}{8\pi}\int_0^{2\pi}  \ln(r_x^2+\varepsilon^2-2r_x \varepsilon\cos(\theta_x-\theta))\ d\theta + \frac{1}{4\pi} \int_0^{2\pi}\int_0^\varepsilon r^3\frac{1-r_x\cos(\theta_x-\theta)}{r_x^2+r^2-2r_x r\cos(\theta_x-\theta)} \ dr\ d\theta\]
    
    \textbullet ~ 3
    
    \[ -\frac{1}{2\pi}\int_0^{2\pi} \int_0^\varepsilon r (\frac{1}{2}\ln \alpha + \ln 2 - \gamma)\ dr\ d\theta = -\frac{\varepsilon^4}{4} \Big(\frac{1}{2}\ln \alpha + \ln 2 - \gamma\Big) \]
    
    \textbullet ~ 4 (TODO)
    
    \[ O(1)\int_0^{2\pi} \int_0^\varepsilon r  (r_x^2+r^2-2r_x r\cos(\theta_x-\theta))|\ln\sqrt{r_x^2+r^2-2r_x r\cos(\theta_x-\theta)}|\ dr\ d\theta \]
\end{proof}

\subsection{strat 2}

On va dire qu'on connait $G_0$ sur tout $\Omega$ mais qu'on peut le calculer explicitement sur $B_\varepsilon$. \\

\begin{proposition}  We have, for $\varepsilon$ small enough,
    \[ \|G_0(\cdot,y)\|_{L^2(B_\varepsilon)} \leq -\frac{1}{2\sqrt{\pi}}\varepsilon\Big(\ln(\varepsilon - r_y) - \frac{1}{2}\ln\alpha - \ln 2 + \gamma\Big) + O\Big(\varepsilon(\varepsilon - r_y)^2|\ln (\varepsilon - r_y)|\Big) \]
\end{proposition}
\begin{proof} Let $y$ in $B_\varepsilon$.

    \[ \|G_0(\cdot,y)\|_{L^2(B_\varepsilon)} \leq \sqrt{\pi}\|G_0(\cdot,y)\|_{L^\infty(B_\varepsilon)}\varepsilon \leq \sqrt{\pi}\|G_0(\cdot,y)\|_{L^\infty(K)}\varepsilon \]
    
    We need to show that $\|G_0(\cdot,y)\|_{L^\infty(K)}$ does not depend on $\varepsilon$, for $\varepsilon$ small enough.
    
    \[ \|G_0(\cdot,y)\|_{L^\infty(K)} := \sup_{x\in K}|G_0(x,y)| = \max\{ \sup_{x\in B_\varepsilon}|G_0(x,y)|, \sup_{x\in K_\varepsilon}|G_0(x,y)| \} \]
    
    \[ = \max\{ \sup_{x\in B_\varepsilon}|G_0(x,y)|, \sup_{x\in K_\varepsilon}|G_p(x,y)| \} \]
    
    \textbullet ~ \[ \sup_{x\in B_\varepsilon}|G_0(x,y)| =  \frac{1}{2\pi}\sup_{x\in B_\varepsilon} | \sum_{n=-\infty}^{+\infty} \frac{I_n(\frac{r_y}{\sqrt{\alpha}}) K_n(\frac{\varepsilon}{\sqrt{\alpha}})}{I_n \Big(\frac{\varepsilon}{\sqrt{\alpha}}\Big)} I_n \Big(\frac{r_x}{\sqrt{\alpha}}\Big)\cos(n(\theta_y-\theta_x)) | \]
    
    $\cos(n(\theta_y-\theta_x))$ is maximal when $\theta_y=\theta_x$. $I_n$ and $K_n$ are positive on $\R^+$. $I_n$ is an increasing function on $\R^+$. Thus, 
    
    \[ \sup_{x\in B_\varepsilon}|G_0(x,y)| =  \frac{1}{2\pi} \sum_{n=-\infty}^{+\infty} I_n(\frac{r_y}{\sqrt{\alpha}}) K_n(\frac{\varepsilon}{\sqrt{\alpha}}) \]
    
    is reached for $r_x=\varepsilon$ and $\theta_x = \theta_y$.
    
    \textbullet ~ \[ \sup_{x\in K_\varepsilon}|G_p(x,y)| = \frac{1}{2\pi}\sup_{x\in K_\varepsilon}|K_0\Big(\frac{1}{\sqrt{\alpha}}|x-y|\Big)| = \frac{1}{2\pi}\sup_{x\in K_\varepsilon}|K_0\Big(\frac{1}{\sqrt{\alpha}}\sqrt{r_x^2 + r_y^2 - 2 r_x r_y\cos(\theta_x - \theta_y)}\Big)| \]
    
    $K_0$ is a decreasing function, then $\sup_{x\in K_\varepsilon}|G_p(x,y)|$ is reached for $x\in K_\varepsilon$, such that $|x-y|$ is minimal. Since $y$ is in $B_\varepsilon$, we choose $\theta_x = \theta_y$, we have, since  $r_y \leq r_x$ \\
    
    \[ \sup_{x\in K_\varepsilon}|G_p(x,y)| = \frac{1}{2\pi}\sup_{x\in K_\varepsilon}|K_0\Big(\frac{r_x - r_y}{\sqrt{\alpha}}\Big)|. \]
    
    It is attains for $r_x = \varepsilon$, i.e.
    
    \[ \sup_{x\in K_\varepsilon}|G_p(x,y)| = \frac{1}{2\pi}|K_0\Big(\frac{\varepsilon - r_y}{\sqrt{\alpha}}\Big)|. \]
    
    \textbullet ~ In both cases, the supremum is attain for $r_x=\varepsilon$ and $\theta_x = \theta_y$ which belongs to $\partial B_\varepsilon$. Thus $\sup_{x\in B_\varepsilon}|G_0(x,y)| = \sup_{x\in K_\varepsilon}|G_p(x,y)|$. We have 
    
    \[ \|G_0(\cdot,y)\|_{L^\infty(K)} = \frac{1}{2\pi}|K_0\Big(\frac{\varepsilon - r_y}{\sqrt{\alpha}}\Big)| = -\frac{1}{2\pi}(\ln(\varepsilon - r_y) - \frac{1}{2}\ln\alpha - \ln 2 + \gamma) + O((\varepsilon - r_y)^2|\ln (\varepsilon - r_y)|) \]
    
    Therefore, we have, for $\varepsilon$ small enough,
    
    \[ \|G_0(\cdot,y)\|_{L^2(B_\varepsilon)} \leq -\frac{1}{2\sqrt{\pi}}\varepsilon\Big(\ln(\varepsilon - r_y) - \frac{1}{2}\ln\alpha - \ln 2 + \gamma\Big) + O\Big(\varepsilon(\varepsilon - r_y)^2|\ln (\varepsilon - r_y)|\Big) \]
  
\end{proof}

-------------------------------------------------------------

\begin{proof} Let $y$ in $B_\varepsilon$.

    --------------------------------------

    The ellipticity of $G$ i.e. $\int_{B_\varepsilon} G(x,y)^2\ dx + \alpha\int_{B_\varepsilon}|\nabla G(x,y)|^2\ dx \geq \beta \|G(\cdot,y)\|_{L^2(B_\varepsilon)}^2$
    
    Gives us 
    
    \[  \|G(\cdot,y)\|_{L^2(B_\varepsilon)}^2 \leq \frac{1}{\beta}(\int_{B_\varepsilon} G(x,y)^2\ dx + \alpha\int_{B_\varepsilon}|\nabla G(x,y)|^2\ dx)  \]
    
    \[ \leq \frac{1}{\beta} \int_{B_\varepsilon} \delta_y(x)G(x,y)\ dx = \frac{1}{\beta} G(y,y)  \]
    
    --------------------------------------

    \[ \|G_0(\cdot,y)\|_{L^2(B_\varepsilon)} \leq \sqrt{\pi}\|G_0(\cdot,y)\|_{L^\infty(B_\varepsilon)}\varepsilon \leq \sqrt{\pi}\|G_0(\cdot,y)\|_{L^\infty(K)}\varepsilon \]
    
    We need to show that $\|G_0(\cdot,y)\|_{L^\infty(K)}$ does not depend on $\varepsilon$, for $\varepsilon$ small enough.
    
    \[ \|G_0(\cdot,y)\|_{L^\infty(K)} := \sup_{x\in K}|G_0(x,y)| = \max\{ \sup_{x\in B_\varepsilon}|G_0(x,y)|, \sup_{x\in K_\varepsilon}|G_0(x,y)| \} \]
    
    \[ = \max\{ \sup_{x\in B_\varepsilon}|G_0(x,y)|, \sup_{x\in K_\varepsilon}|G_p(x,y)| \} \]
    
    \textbullet ~ \[ \sup_{x\in B_\varepsilon}|G_0(x,y)| =  \frac{1}{2\pi}\sup_{x\in B_\varepsilon} | \sum_{n=-\infty}^{+\infty} \frac{I_n(\frac{r_y}{\sqrt{\alpha}}) K_n(\frac{\varepsilon}{\sqrt{\alpha}})}{I_n \Big(\frac{\varepsilon}{\sqrt{\alpha}}\Big)} I_n \Big(\frac{r_x}{\sqrt{\alpha}}\Big)\cos(n(\theta_y-\theta_x)) | \]
    
    $\cos(n(\theta_y-\theta_x))$ is maximal when $\theta_y=\theta_x$. $I_n$ and $K_n$ are positive on $\R^+$. $I_n$ is an increasing function on $\R^+$. Thus, 
    
    \[ \sup_{x\in B_\varepsilon}|G_0(x,y)| =  \frac{1}{2\pi} \sum_{n=-\infty}^{+\infty} I_n(\frac{r_y}{\sqrt{\alpha}}) K_n(\frac{\varepsilon}{\sqrt{\alpha}}) \]
    
    is reached for $r_x=\varepsilon$ and $\theta_x = \theta_y$.
    
    \textbullet ~ \[ \sup_{x\in K_\varepsilon}|G_p(x,y)| = \frac{1}{2\pi}\sup_{x\in K_\varepsilon}|K_0\Big(\frac{1}{\sqrt{\alpha}}|x-y|\Big)| = \frac{1}{2\pi}\sup_{x\in K_\varepsilon}|K_0\Big(\frac{1}{\sqrt{\alpha}}\sqrt{r_x^2 + r_y^2 - 2 r_x r_y\cos(\theta_x - \theta_y)}\Big)| \]
    
    $K_0$ is a decreasing function, then $\sup_{x\in K_\varepsilon}|G_p(x,y)|$ is reached for $x\in K_\varepsilon$, such that $|x-y|$ is minimal. \\
    
    1 - If $y$ is in $K_\varepsilon$, $\sup_{x\in K_\varepsilon}|G_p(x,y)| = +\infty$, for $x=y$. \\ 
    
    2 - If $y$ is in $B_\varepsilon$, we choose $\theta_x = \theta_y$, we have, since  $r_y \leq r_x$ \\
    
    \[ \sup_{x\in K_\varepsilon}|G_p(x,y)| = \frac{1}{2\pi}\sup_{x\in K_\varepsilon}|K_0\Big(\frac{r_x - r_y}{\sqrt{\alpha}}\Big)|. \]
    
    It is attains for $r_x = \varepsilon$, i.e.
    
    \[ \sup_{x\in K_\varepsilon}|G_p(x,y)| = \frac{1}{2\pi}|K_0\Big(\frac{\varepsilon - r_y}{\sqrt{\alpha}}\Big)|. \]
    
    3 - If $y$ is in $\Omega\setminus K$, we choose $\theta_x = \theta_y$, we have, since  $r_x \leq r_y$ \\
    
    \[ \sup_{x\in K_\varepsilon}|G_p(x,y)| = \frac{1}{2\pi}\sup_{x\in K_\varepsilon}|K_0\Big(\frac{r_y - r_x}{\sqrt{\alpha}}\Big)| \]
    
    We define $K^\varepsilon := \{ x+y\ \Big|\ x\in K,\ |y|\leq \varepsilon\}$.
    
    ~ 3.1 - $y$ is in $K^\varepsilon$, sup is "the same" than if $y\in B_\varepsilon$.
    
    ~ 3.2 - Independent to $\varepsilon$ but to small compared with other terms when $\varepsilon$ tends to $0$.
\end{proof}

Last proposition \\

\begin{proposition}
    \[ \int_{B_\varepsilon} w(x)\ dx = -\pi^{3/2} g(y_0) \varepsilon^4\ln\varepsilon + O(\varepsilon^4\ln\varepsilon), \]
    when $\varepsilon$ tends to $0$.
\end{proposition}
\begin{proof}
    \[ \int_{B_\varepsilon} w(x)\ dx = \int_{B_\varepsilon} \int_{B_\varepsilon} g(y)G(x,y)\ dy\ dx \]
        
    Fubini,    
        
    \[ \int_{B_\varepsilon} w(x)\ dx = \int_{B_\varepsilon} g(y) \int_{B_\varepsilon}G(x,y)\ dx\ dy \]
    
    Cauchy-Schwarz
    
    \[ \int_{B_\varepsilon} w(x)\ dx \leq \pi\varepsilon^2\int_{B_\varepsilon} g(y) \|G(\cdot,y)\|_{L^2(B_\varepsilon)}\ dy \]
    
    Minkowsky
    
    \[ \int_{B_\varepsilon} w(x)\ dx \leq \underbrace{ \pi\varepsilon^2\int_{B_\varepsilon} g(y) \|G_0(\cdot,y)\|_{L^2(B_\varepsilon)}\ dy}_{ =: I_1} + \underbrace{\pi\varepsilon^2\int_{B_\varepsilon} g(y) \|G_\text{p}(\cdot,y)\|_{L^2(B_\varepsilon)}\ dy}_{=: I_2} \]
    
    \textbullet ~ 
    
    \[ I_1 \leq \pi\varepsilon^2\int_{B_\varepsilon} g(y) (-\frac{1}{2\sqrt{\pi}}\varepsilon\Big(\ln(\varepsilon - r_y) - \frac{1}{2}\ln\alpha - \ln 2 + \gamma\Big) + O\Big(\varepsilon(\varepsilon - r_y)^2|\ln (\varepsilon - r_y)|\Big))\ dy \]
    
    \[ I_1 \leq -\frac{\sqrt{\pi}}{2}\varepsilon^3\int_{B_\varepsilon} g(y)\Big(\ln(\varepsilon - r_y) - \frac{1}{2}\ln\alpha - \ln 2 + \gamma\Big)\ dy + O(1)\varepsilon^3\int_{B_\varepsilon} g(y)(\varepsilon - r_y)^2|\ln (\varepsilon - r_y)|\ dy \]
    
    \[ \leq -\pi^{3/2} g(y_0) \varepsilon^4\ln\varepsilon + O(\varepsilon^4). \]
    
    Thus,
    
    \[ I_1  = O(\varepsilon^4\ln\varepsilon) \]
    
    \textbullet ~ 
    
    \[ I_2 = \pi\varepsilon^2\int_{B_\varepsilon}\int_{B_\varepsilon} g(y) (-\frac{1}{2\pi}\Big(\ln|x-y| + \frac{1}{2}\ln \alpha + \ln 2 - \gamma\Big) + O(|x-y|^2|\ln|x-y||))\ dy \]
    
    \[ = -\pi^{3/2} g(y_0) \varepsilon^4\ln\varepsilon + O(\varepsilon^4). \]
    
\end{proof}
