# Supplementary material for: Choosing The Best Interpolation Data in Images with Noise
Source: arXiv:2011.02363 source file (2020-11-04)
Supplement: Supplementary file 2 [file appendix04.tex]

\section{Draft 2}

\subsection{Denoising by Inpainting}

To denoise an image, one can use Bayesian approach like in Section \ref{sec:gaussian-noise}, that is

\[ \min_{f\in [0,1]^N} \|g-f\|_2^2, \]

where $g$ is the noisy input image. In such method, we do not impose the processed image $f$ to be equals to the noised image $g$ on some part. However, by using the methods presented in this paper, we minimize the $L^2$-error between the input image and the reconstructed image, like in the Bayesian case, but we also impose the processed image to be equals to the noised image on some part, $K\subset D$. It implies the following : If we take too few pixels, the reconstruction will, of course be bad. However, if we take too much pixels, the output image will be close to the input image, namely the noisy image, and consequently will be noisy as well. In this section, we will use inpainting to denoise an image as explained in \cite{denoisingbyinpainting}. We compare our proposed methods to the Linear Diffusion Filter which is known to denoise image \cite{diffusionfilter}.

\begin{figure}[H]
	\centering
	\subfloat[Original image, $f$.]{
		\includegraphics[height=3.5cm]{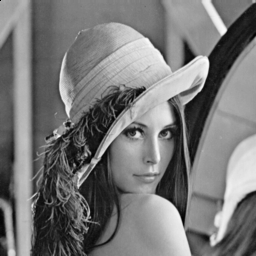}
	}
	\qquad
	\subfloat[Input image with $\sigma = 0.05$, $f_\text{n}$. $\|f_\text{n}-f\|_{L^2(D)}=12.51$.]{
		\includegraphics[height=3.5cm]{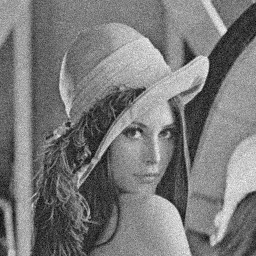}
	}
	\qquad
	\subfloat[Linear diffusion filter at $\sigma=0.6$, $u$. $\|u-f\|_{L^2(D)}=9.25$.]{
		\includegraphics[height=3.5cm]{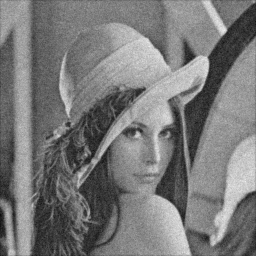}
	}
	\qquad
	\subfloat[``L2Const'' with $\alpha=100$ and $c=0.25$, $u$. $\|u-f\|_{L^2(D)}=9.51$.]{
		\includegraphics[height=3.5cm]{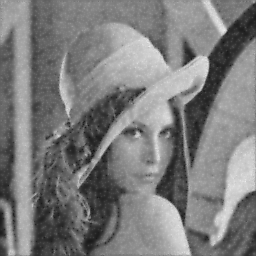}
	}
	\qquad
	\subfloat[``L2Sta'' with thresholding, $\alpha=30$ and $c=0.3$ and $N=50$, $u$. $\|u-f\|_{L^2(D)}=9.20$.]{
		\includegraphics[height=3.5cm]{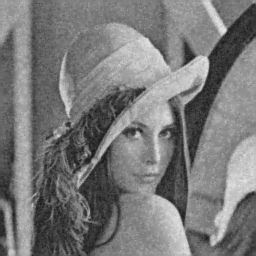}
	}
	\qquad
	\subfloat[``L2Dec'', $\alpha=1$ and $c=0.22$ and $dc=0.98$, $u$. $\|u-f\|_{L^2(D)}=9.23$.]{
		\includegraphics[height=3.5cm]{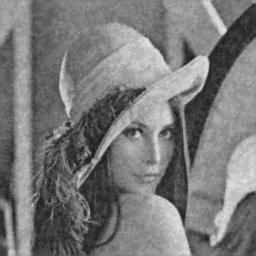}
	}
	\qquad
	\subfloat[``L2Inc'', $\alpha=18$ and $c=0.22$ and $N=40$, $u$. $\|u-f\|_{L^2(D)}=8.73$.]{
		\includegraphics[height=3.5cm]{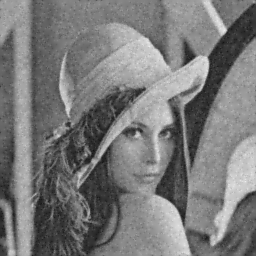}
	}
	
	\caption{.}
	\label{fig:experiments:method:denoising}
\end{figure} 

\subsection{Evolution of the Solution Over Time}

As shown in Figure \ref{fig:experiments:evolution}, we notice than, for well chosen parameters, during the encoding step, the error between the original image $f$ and the solution $u_n$ decreases until being lower than the error between the original image $f$ and the noised one $f_\text{n}$. This motives us to perform a small change in our encoding methods : Instead of solving Problem \ref{pb:problem_1_time_implicit}, we solve the following one

\begin{problem} For $n\in\N$, by knowing $u^n$, find $u^{n+1}$ in $H^1(D)$ such that
	\begin{equation}
		\left\{\begin{array}{rl}
			u^{n+1} - \delta t \alpha \Delta u^{n+1} = u^n, & \text{in}\ D\setminus K_n, \\
			u^{n+1} = u_n, & \text{in}\ K_n, \\
			\frac{\partial u^{n+1}}{\partial \mathbf{n}} = 0, & \text{on}\ \partial D, \\
		\end{array}\right .\label{eq:problem_1_time_implicit_denoising}
	\end{equation}
	
	and
	
	\begin{equation*}
		\left\{\begin{array}{rl}
		    & u^0 = f, \\
		    & K_0 \subset D.
		\end{array}\right .
	\end{equation*}

	\label{pb:problem_1_time_implicit_denoising}
\end{problem}

Moreover, for the decoding step, we use the mask as usual and $u_N$ instead of $f$. Since in reality we have $f_\text{n}$ instead of $f$, we replace $f$ in Problem \ref{pb:problem_1_time_implicit} by $u_n$ in $K_n$, which apears to be closer to $f$ than $f_\text{n}$ is and thus, impose $u_0 = f$.

\begin{figure}[H]
	\centering
	\subfloat[$N=5$, $\alpha=18$]{
		\includegraphics[height=3.5cm]{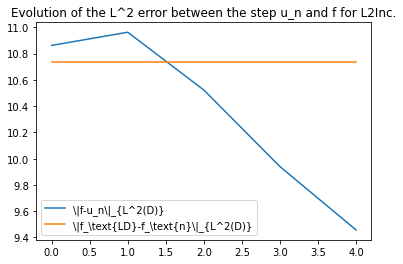}
	}
	\qquad
	\subfloat[$N=10$, $\alpha=18$]{
		\includegraphics[height=3.5cm]{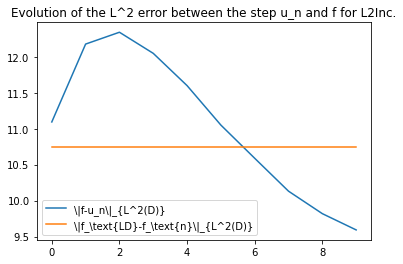}
	}
	\qquad
	\subfloat[$N=40$, $\alpha=18$]{
		\includegraphics[height=3.5cm]{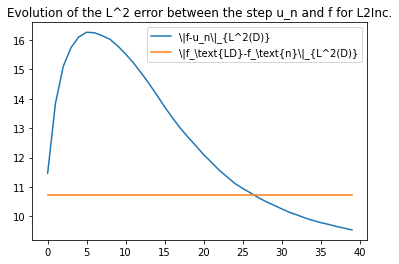}
	}
	\qquad
	\subfloat[$N=10$, $\alpha=5$]{
		\includegraphics[height=3.5cm]{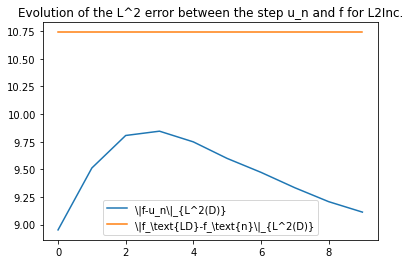}
	}
	
	\caption{L2Inc $c=0.1$, $f_\text{LD}$ is the Linear Diffusion of $f$ for $\sigma = 1'$.}
	\label{fig:experiments:evolution}
\end{figure} 

Figure \ref{fig:experiments:method:denoising-modif} are examples of reconstructed image with the new method

\begin{figure}[H]
	\centering
	\subfloat[Original image, $f$.]{
		\includegraphics[height=3.5cm]{resources/images/Lenna.png}
	}
	\qquad
	\subfloat[Input image with $\sigma = 0.05$, $f_\text{n}$. $\|f_\text{n}-f\|_{L^2(D)}=12.51$.]{
		\includegraphics[height=3.5cm]{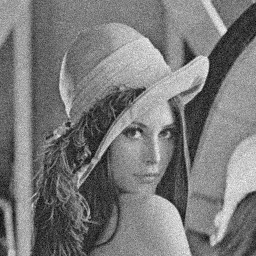}
	}
	\qquad
	\subfloat[Linear diffusion filter at $\sigma=0.6$, $u$. $\|u-f\|_{L^2(D)}=9.25$.]{
		\includegraphics[height=3.5cm]{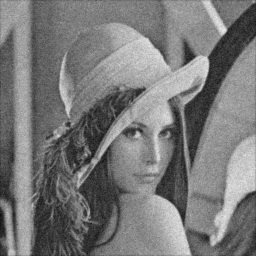}
	}
	\qquad
	\subfloat[``L2Inc'', $\alpha=5$ and $c=0.22$ and $N=6$, $u$. $\|u-f\|_{L^2(D)}=10.47$.]{
		\includegraphics[height=3.5cm]{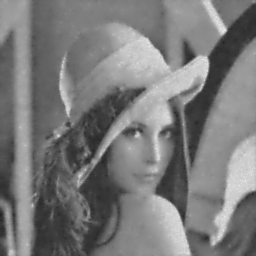}
	}
	\qquad
	\subfloat[``L2Insta'', $\alpha=5$ and $c=0.22$ and $N=5$, $u$. $\|u-f\|_{L^2(D)}=9.33$.]{
		\includegraphics[height=3.5cm]{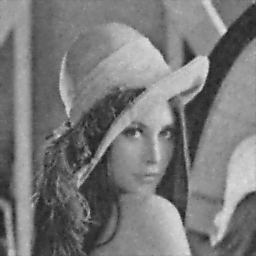}
	}
	
	\caption{.}
	\label{fig:experiments:method:denoising-modif}
\end{figure}
